# Supplementary material for: Understanding the Humans Behind Online Misinformation: An Observational Study Through the Lens of the COVID-19 Pandemic
Source: arXiv:2310.08483 source file (2024-01-18)
Supplement: Supplementary file 1 [file appendix.tex]

\appendix

\section{Discussion on Misclassifications}
\label{sec:misclassification_cost}

Our work employs an automated data labeling methodology using trained machine learning classifiers. While, these classifiers perform well over the used metrics (Accuracy, Precision etc; ref. Table~\ref{tab:classifier_performance}), we acknowledge that inaccuracies in the classification process may still arise, particularly for challenging cases. Our study tries to address this potential issue by conducting our analysis at the user level, as opposed to the post level, while also applying empirically-driven appropriate thresholds pertaining to the number and ratio of misinformative tweets (as mentioned in Section~\ref{sec:data_collection_clasification}). Through the implementation of these thresholds for user-level classification, we ensure the robustness of our analytical approach against misclassifications produced by the classifiers. Although our study's design has been structured to establish a high degree of robustness, it is important to acknowledge the possibility of occasional misclassifications at the user level. Nevertheless, it is noteworthy that the overarching findings of this study are expected to exhibit consistency and similarity when examined at an aggregated level.

\section{Potential Misuse and Negative Impact on Society}
\label{sec:negative_impact}

Our study is centered on the examination of user behavior, with a specific focus on investigating the correlation between users' historical tendencies in disseminating misinformation and their present behavior in this regard. Consequently, there exists a conceivable risk of misusing the insights from our work if users on social media platforms are subject to biased tracking solely based on their current behaviors, particularly regarding the anticipation of future misinformation sharing. The act of de-platforming users predicated on such anticipations has the potential to limit users' freedom of expression.
